# Supplementary material for: GARDENIA: A Domain-specific Benchmark Suite for Next-generation Accelerators
Source: arXiv:1708.04567 source file (2018-02-03)
Supplement: Supplementary file 1 [file appendix.tex]

% Appendix
\appendix
\section{Switching Times}

In this appendix, we measure the channel switching time of Micaz
\cite{CROSSBOW} sensor devices.  In our experiments, one mote
alternatingly switches between Channels~11 and~12. Every time after
the node switches to a channel, it sends out a packet immediately and
then changes to a new channel as soon as the transmission is finished.
We measure the number of packets the test mote can send in 10 seconds,
denoted as $N_{1}$. In contrast, we also measure the same value of the
test mote without switching channels, denoted as $N_{2}$. We calculate
the channel-switching time $s$ as
\begin{displaymath}%
s=\frac{10}{N_{1}}-\frac{10}{N_{2}}.
\end{displaymath}%
By repeating the experiments 100 times, we get the average
channel-switching time of Micaz motes: 24.3\,$\mu$s.

\section{Supplementary Materials}

\begin{printonly}
  See the supplementary materials in the online version
\end{printonly}

\begin{screenonly}
\subsection{This is an Example of Appendix Subsection Head}

Channel-switching time is measured as the time length it takes for
motes to successfully switch from one channel to another. This
parameter impacts the maximum network throughput, because motes
cannot receive or send any packet during this period of time, and it
also affects the efficiency of toggle snooping in MMSN, where motes
need to sense through channels rapidly.

By repeating experiments 100 times, we get the average
channel-switching time of Micaz motes: 24.3 $\mu$s. We then conduct
the same experiments with different Micaz motes, as well as
experiments with the transmitter switching from Channel 11 to other
channels. In both scenarios, the channel-switching time does not have
obvious changes. (In our experiments, all values are in the range of
23.6 $\mu$s to 24.9 $\mu$s.)

\subsection{Appendix Subsection Head}

The primary consumer of energy in WSNs is idle listening. The key to
reduce idle listening is executing low duty-cycle on nodes. Two
primary approaches are considered in controlling duty-cycles in the
MAC layer.
  
\end{screenonly}

\begin{acks}

The authors would like to thank Dr. Maura Turolla of Telecom
Italia for providing specifications about the application scenario.

The work is supported by the \grantsponsor{GS501100001809}{National
  Natural Science Foundation of
  China}{http://dx.doi.org/10.13039/501100001809} under Grant
No.:~\grantnum{GS501100001809}{61273304\_a}
and~\grantnum[http://www.nnsf.cn/youngscientsts]{GS501100001809}{Young
  Scientsts' Support Program}.

\end{acks}
